# Supplementary material for: What is the right addressing scheme for India?
Source: arXiv:1801.06540 source file (2018-01-28)
Supplement: Supplementary file 1 [file appendix.tex]

\section*{APPENDIX}
\begin{enumerate}
    \item THE ECONOMIC COST OF POOR ADDRESSES
    
    Our estimate from the top three industries indicate that poor addresses cost India \$10-14B annually, ~0.5\% of the GDP; see Table 3. \par
    \begin{minipage}{\linewidth}
    \centering
    \includegraphics[width=\textwidth]{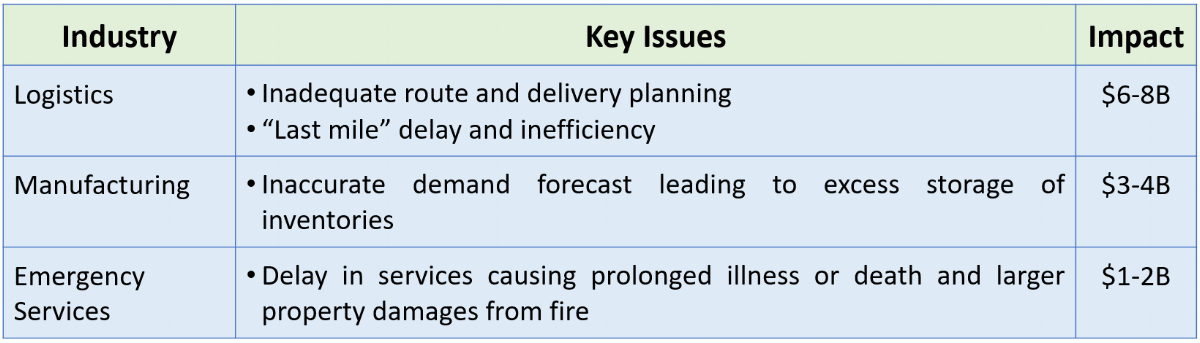}
    \captionof{table}{The economic cost of bad addresses in India}
    \end{minipage}
    
    Note that the numbers presented in Table A1 capture the cost of bad addresses, but do not include additional benefits of having better addresses: rising productivity and income gains, which lead to further growth of businesses etc.
    
    \item COMBINATORICS OF MACHINE CODES
    \begin{enumerate}
        \item \textbf{What3Words}: An arrangement of 3 random words is assigned to each of roughly 57 trillion imaginary 3m x 3m grids on the surface of the Earth. Each W3W code is derived from a static list of 40,000 English words, from which 3 words are chosen at random and ordered in all possible ways. This generates a total of 40,000C3  x 3! \texttt{\char`\~} 64 trillion unique arrangements.
        
        \item \textbf{Zippr/eLoc}: Both of these schemes assign a random alphanumeric string to each address in India. Assume that the minimum length required for such a short-code is n characters, which must be randomly drawn from a pool of 26 alphabets and 10 numerals. In order to assign short-codes for roughly 300 million households, the value of n can be worked out by solving 36Cn x n! \texttt{\char`\~} 36\^{}n\textgreater 3 x 10\^{}8. Using log transformation, we get n $\geq$ 6.
        
        \item \textbf{Plus Codes}: An alphanumeric code is assigned to each of roughly 57 trillion imaginary 3m x 3m grids on the surface of the Earth. Using the above logic, the value of n can be worked out by solving 36\^{}n\textgreater 5.7 x 10\^{}13. We obtain n $\geq$ 9, however, since Plus Codes maintain a hierarchy in the codes, they require up to 11 characters.
    \end{enumerate}
\end{enumerate}
